# Supplementary material for: Making Logic Learnable With Neural Networks
Source: arXiv:2002.03847 source file (2020-06-07)
Supplement: Supplementary file 1 [file 10_supplementary_old.tex]

\clearpage
\section*{Appendix}
\label{appendix}

% -------------------------------------------------------
\subsection{Further Results}
\label{further_results}

The results of a broad experimental setup with multiple parameters can be found in the tables on the following pages (Table \ref{lgn_eighttotal_results}, \ref{rf_eighttotal_results}, \ref{minisat_result}, \ref{lgn_thirtytwototal_results} and \ref{rf_thirtytwototal_results}). \\

The evaluation of our methods is based on the following assumptions and limitations. We only use fully-connected neural networks which we train with Adam optimizer \cite{adam}. For the GI bleeding data set, our architecture follows the one used in a broad evaluation of machine learning models on the same data set \cite{shung2020validation}, which showed state-of-the-art results and was built out of only one hidden layer with 20 nodes. For training the real-valued neural network, we use a ReLU activation function on the input layer and on all hidden layers, while using a softmax activation function on the last layer in combination with a cross-entropy loss function. The ReLU activation function is also modeled within the logic of intermediate layers, but for the logic representation of the last layer, we use an identity mapping, followed by an argmax-function to get the final class prediction. This is done to prevent issues related to an exact approximation of the softmax function. Moreover we create only combinational circuits and leave the analysis and optimization of the timing aspects of the circuits as future work. Within the logic we make the assumtion that the multiplier entities have the double bit width as the number of total bits used in the data-, the activation- and the weight-quantization scheme (see Section \ref{quantization}). Similarly, we assume all accumulator entities (which do the summations) to have three times of the bit width as the quantization scheme. 

% -------------------------------------------------------
\subsection{Interpretable Reports}
\label{reports}

In the following, we provide an example of how reports from the logic can look like. We derive the report for a single node $l0;n0$ of the first layer from a direct translation of a neural network to arithmetic logic. It receives four input features from the data: the systolic blood pressure, the haemoglobin level, the urea level and the creatinine level. The inputs and the activations are quantized to 4 total bits and 2 fractional bits. The Boolean equations derived from the AIG of the logic module can be found in the following. Also a single logic module can potentially be simulated, using this report. The derived AIG has 134 nodes and can be visualized as shown in Figure \ref{l0n0_figure}. From this is can be quickly seen that in this example there is no dependence on the variables creatinine and urea, which means that they are internally treated as don't-cares. Similar reports can be created from any arbitrary concatenation of logic modules, allowing simulations and interpretations also of only intermediate layers or nodes or measuring variables' influences.

% \newpage
\textbf{Logic Report:} l0n0{\_}nn\\
\noindent\rule{\columnwidth}{0.4pt}

\textbf{Inputs:}\\
\noindent\rule{\columnwidth}{0.4pt}

Input 0:	systolic\\
Input 1:	haemoglobin\\
Input 2:	urea\\
Input 3:	creatinine\\

\textbf{Outputs:}\\
\noindent\rule{\columnwidth}{0.4pt}

Output:	l0n0{\_}nn{\_}out\\

\textbf{Equations:}\\
\noindent\rule{\columnwidth}{0.4pt}

n21 = systolic[0] AND systolic[1];\\
n22 = NOT systolic[0] AND NOT systolic[1];\\
n23 = NOT n21 AND NOT n22;\\
n24 = haemoglobin[0] AND n23;\\
n25 = systolic[2] AND n23;\\
n26 = NOT systolic[2] AND NOT n23;\\
n27 = NOT n25 AND NOT n26;\\
n28 = n21 AND n27;\\
n29 = NOT n21 AND NOT n27;\\
n30 = NOT n28 AND NOT n29;\\
n31 = haemoglobin[0] AND haemoglobin[1];\\
n32 = NOT haemoglobin[0] AND NOT haemoglobin[1];\\
n33 = NOT n31 AND NOT n32;\\
n34 = n30 AND n33;\\
n35 = NOT n30 AND NOT n33;\\
n36 = NOT n34 AND NOT n35;\\
n37 = n24 AND n36;\\
n38 = NOT n24 AND NOT n36;\\
n39 = NOT n37 AND NOT n38;\\
n40 = NOT systolic[0] AND systolic[1];\\
n41 = systolic[0] AND NOT systolic[1];\\
n42 = NOT n40 AND NOT n41;\\
n43 = systolic[2] AND n42;\\
n44 = NOT systolic[2] AND NOT n42;\\
n45 = NOT n43 AND NOT n44;\\
n46 = n21 AND n45;\\
n47 = NOT n21 AND NOT n45;\\
n48 = NOT n46 AND NOT n47;\\
n49 = NOT systolic[3] AND n48;\\
n50 = NOT n25 AND NOT n28;\\
n51 = systolic[3] AND NOT n48;\\
n52 = NOT n49 AND NOT n51;\\
n53 = NOT n50 AND n52;\\
n54 = NOT n49 AND NOT n53;\\
n55 = NOT n43 AND NOT n46;\\
n56 = NOT systolic[1] AND systolic[2];\\
n57 = systolic[1] AND NOT systolic[2];\\
n58 = NOT n56 AND NOT n57;\\
n59 = n40 AND n58;\\
n60 = NOT n40 AND NOT n58;\\
n61 = NOT n59 AND NOT n60;\\
n62 = NOT systolic[3] AND n61;\\
n63 = systolic[3] AND NOT n61;\\
n64 = NOT n62 AND NOT n63;\\
n65 = NOT n55 AND n64;\\
n66 = n55 AND NOT n64;\\
n67 = NOT n65 AND NOT n66;\\
n68 = n54 AND NOT n67;\\
n69 = NOT n54 AND n67;\\
n70 = NOT n68 AND NOT n69;\\
n71 = NOT haemoglobin[0] AND haemoglobin[1];\\
n72 = haemoglobin[0] AND NOT haemoglobin[1];\\
n73 = NOT n71 AND NOT n72;\\
n74 = haemoglobin[2] AND n73;\\
n75 = NOT haemoglobin[2] AND NOT n73;\\
n76 = NOT n74 AND NOT n75;\\
n77 = n31 AND n76;\\
n78 = NOT n31 AND NOT n76;\\
n79 = NOT n77 AND NOT n78;\\
n80 = NOT n74 AND NOT n77;\\
n81 = NOT haemoglobin[1] AND haemoglobin[2];\\
n82 = haemoglobin[1] AND NOT haemoglobin[2];\\
n83 = NOT n81 AND NOT n82;\\
n84 = n71 AND n83;\\
n85 = NOT n71 AND NOT n83;\\
n86 = NOT n84 AND NOT n85;\\
n87 = NOT haemoglobin[3] AND n86;\\
n88 = haemoglobin[3] AND NOT n86;\\
n89 = NOT n87 AND NOT n88;\\
n90 = NOT n80 AND n89;\\
n91 = n80 AND NOT n89;\\
n92 = NOT n90 AND NOT n91;\\
n93 = NOT n79 AND NOT n92;\\
n94 = n79 AND n92;\\
n95 = NOT n93 AND NOT n94;\\
n96 = NOT n70 AND NOT n95;\\
n97 = n50 AND NOT n52;\\
n98 = NOT n53 AND NOT n97;\\
n99 = NOT n79 AND n98;\\
n100 = NOT n34 AND NOT n37;\\
n101 = n79 AND NOT n98;\\
n102 = NOT n99 AND NOT n101;\\
n103 = NOT n100 AND n102;\\
n104 = NOT n99 AND NOT n103;\\
n105 = n70 AND n95;\\
n106 = NOT n96 AND NOT n105;\\
n107 = NOT n104 AND n106;\\
n108 = NOT n96 AND NOT n107;\\
n109 = NOT n62 AND NOT n65;\\
n110 = NOT n56 AND NOT n59;\\
n111 = NOT systolic[2] AND NOT systolic[3];\\
n112 = systolic[2] AND systolic[3];\\
n113 = NOT n111 AND NOT n112;\\
n114 = NOT n110 AND n113;\\
n115 = n110 AND NOT n113;\\
n116 = NOT n114 AND NOT n115;\\
n117 = NOT n109 AND n116;\\
n118 = n109 AND NOT n116;\\
n119 = NOT n117 AND NOT n118;\\
n120 = NOT n68 AND n119;\\
n121 = n68 AND NOT n119;\\
n122 = NOT n120 AND NOT n121;\\
n123 = NOT n87 AND NOT n90;\\
n124 = NOT n81 AND NOT n84;\\
n125 = NOT haemoglobin[2] AND NOT haemoglobin[3];\\
n126 = haemoglobin[2] AND haemoglobin[3];\\
n127 = NOT n125 AND NOT n126;\\
n128 = NOT n124 AND n127;\\
n129 = n124 AND NOT n127;\\
n130 = NOT n128 AND NOT n129;\\
n131 = NOT n123 AND n130;\\
n132 = n123 AND NOT n130;\\
n133 = NOT n131 AND NOT n132;\\
n134 = NOT n93 AND n133;\\
n135 = n93 AND NOT n133;\\
n136 = NOT n134 AND NOT n135;\\
n137 = n122 AND n136;\\
n138 = NOT n122 AND NOT n136;\\
n139 = NOT n137 AND NOT n138;\\
n140 = NOT n108 AND n139;\\
n141 = n108 AND NOT n139;\\
n142 = NOT n140 AND NOT n141;\\
n143 = n104 AND NOT n106;\\
n144 = NOT n107 AND NOT n143;\\
n145 = n100 AND NOT n102;\\
n146 = NOT n103 AND NOT n145;\\
n147 = NOT n39 AND NOT n146;\\
n148 = NOT n144 AND n147;\\
n149 = NOT n142 AND n148;\\
n150 = NOT n142 AND NOT n149;\\
l0n0{\_}nn{\_}out[0] = n39 AND n150;\\
l0n0{\_}nn{\_}out[1] = n146 AND n150;\\
l0n0{\_}nn{\_}out[2] = n144 AND n150;\\
l0n0{\_}nn{\_}out[3] = n142 AND n150;\\

% -------------------------------------------------------
\begin{figure*}[ht]
\vskip 0.2in
\begin{center}
\centerline{\includegraphics[width=\textwidth]{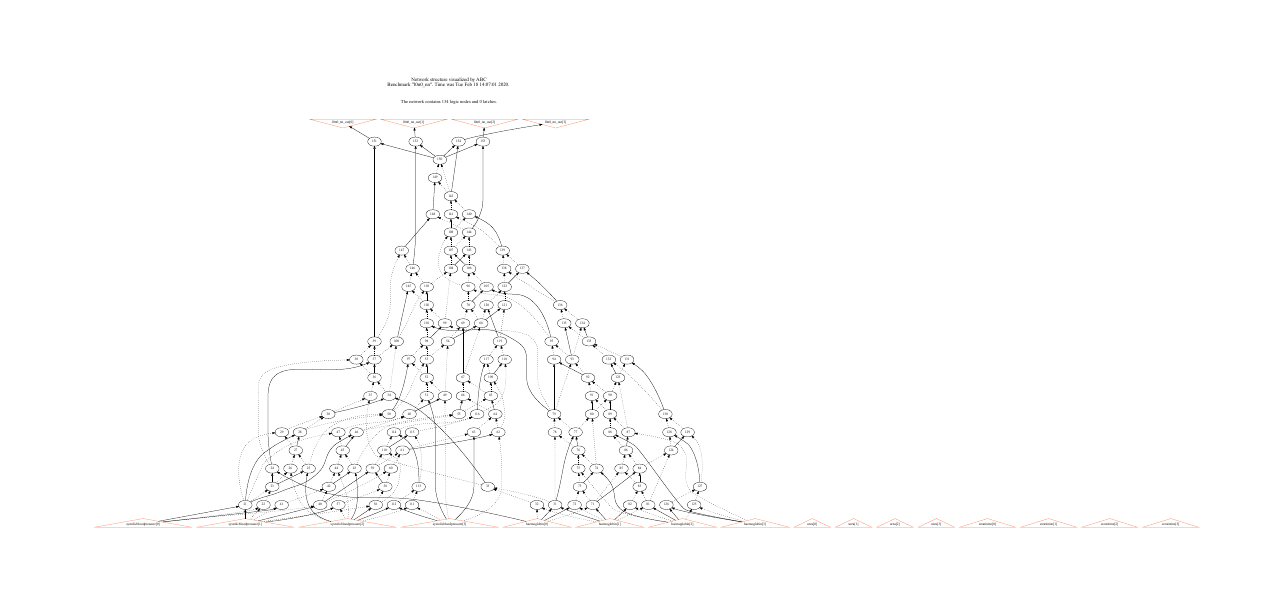}}
\caption{Example of the AIG that is derived from a simple logic module. The visualization was exported after creating the AIG with ABC \cite{abc}.}
\label{l0n0_figure}
\end{center}
\vskip -0.2in
\end{figure*}

% -------------------------------------------------------
\begin{table*}[ht]
\caption{Results of \textbf{LogicNet} as intermediate step with the logic being quantized to \textbf{8 total bits and 6 fractional bits}. The column-wise ``winner" is marked in bold.}
\label{lgn_eighttotal_results}
\vskip 0.15in
\begin{center}
% \begin{small}
\begin{sc}
\scalebox{0.8}{
\begin{tabular}{ccccccc}
\toprule
Depth & Width & LUT-Size & AIG Nodes & AIG Levels & Logic Accuracy (\%) \\
\midrule
2 & 50 & 4 & 80,756 & 187 & 54.17 \\
2 & 100 & 4 & 71,162 & 186 & 54.00 \\
2 & 200 & 4 & \textbf{56,738} & \textbf{184} & 54.17 \\
2 & 50 & 6 & 107,190 & 188 & 54.17 \\
2 & 100 & 6 & 116,563 & 188 & 54.17 \\
2 & 200 & 6 & 176,307 & 204 & 54.17 \\
2 & 50 & 8 & 224,670 & 202 & 53.50 \\ 
2 & 100 & 8 & 217,562 & 204 & 54.33 \\ 
2 & 200 & 8 & 135,649 & 189 & 54.00 \\ 
% \midrule
3 & 50 & 4 & 239,243 & 205 & 53.50 \\ 
3 & 100 & 4 & 221,350 & 201 & 53.83 \\ 
3 & 200 & 4 & 215,211 & 206 & 54.17 \\ 
3 & 50 & 6 & 146,347 & 192 & 56.50 \\ 
3 & 100 & 6 & 249,995 & 203 & 54.00 \\ 
3 & 200 & 6 & 147,908 & 196 & 54.33 \\
3 & 50 & 8 & 149,378 & 197 & 54.17 \\
3 & 100 & 8 & 147,145 & 195 & 55.83 \\
3 & 200 & 8 & 149,399 & 196 & 54.17 \\
% \midrule
4 & 50 & 4 & 146,130 & 192 & 54.33 \\ 
4 & 100 & 4 & 146,592 & 191 & 54.17 \\ 
4 & 200 & 4 & 145,878 & 191 & 50.33 \\ 
4 & 50 & 6 & 254,011 & 209 & 54.67 \\ 
4 & 100 & 6 & 151,359 & 197 & 54.17 \\
4 & 200 & 6 & 255,886 & 205 & \textbf{58.83} \\
4 & 50 & 8 & 255,403 & 209 & 54.33 \\ 
4 & 100 & 8 & 256,910 & 212 & 56.00 \\ 
4 & 200 & 8 & 157,274 & 201 & 57.33 \\
\bottomrule
\end{tabular}
}
\end{sc}
\end{center}
\end{table*}

% -------------------------------------------------------
\begin{table*}[ht]
\caption{Results of \textbf{random forest} as intermediate step with the logic being quantized to \textbf{8 total bits and 6 fractional bits}. The column-wise ``winner" is marked in bold.}
\label{rf_eighttotal_results}
\vskip 0.15in
\begin{center}
\begin{sc}
\scalebox{0.8}{
\begin{tabular}{cccccc}
\toprule
Estimators & Max. Depth & AIG Nodes & AIG Levels & Logic Accuracy (\%) \\
% \midrule
2 & 5 & \textbf{198,378} & \textbf{227} & 54.17 \\
2 & 10 & 541,789 & 251 & 48.50 \\
2 & 15 & 472,091 & 261 & 53.50 \\
% \midrule
3 & 5 & 341,500 & 272 & 52.50 \\
3 & 10 & 737,429 & 263 & 52.00 \\
3 & 15 & 630,701 & 275 & 54.17 \\
% \midrule
4 & 5 & 266,826 & 252 & \textbf{55.00} \\
4 & 10 & 912,589 & 275 & 49.83 \\
4 & 15 & 793,930 & 287 & 48.83 \\
\bottomrule
\end{tabular}
}
\end{sc}
\end{center}
\vskip -0.1in
\end{table*}

% -------------------------------------------------------

\begin{table*}[ht]
\caption{Results of the computing times for MiniSAT \cite{een2003extensible} to find satisfying arguments for multiple settings of bloated and reduced logic - ordered by the number of AIG nodes.}
\label{minisat_result}
\vskip 0.15in
\begin{center}
% \begin{small}
\begin{sc}
\scalebox{0.8}{
\begin{tabular}{cccccc}
\toprule
Logic Translation \\($m$ total bits, $i$ fractional bits) & Settings & AIG Nodes & AIG Levels & MiniSAT time \\
\midrule
Neural Network ($32$, $16$) & - & 2,516,251 & 1,113 & 18,813.05 s (313.55 min) \\ % 01
Random Forest ($8$, $6$) & Estimators: 4; Max. Depth: 10 & 912,589 & 275 & 22,310.16 s (371.84 min) \\ % 03
LogicNet ($8$, $6$) & Depth: 4; Width: 100; LUT-Size: 8 & 256,910 & 212 & 1,264.43 s (21.07 min) \\ %AIG Opt. ! % 02
Neural Network ($8$, $4$) & - & 210,457 & 477 & 76.08 s (1.27 min) \\ % 06
Random Forest ($8$, $6$) & Estimators: 2; Max. Depth: 5 & 198,378 & 227 & 5,226.24 s (87.10 min) \\ % 05
LogicNet ($8$, $6$) & Depth: 2; Width: 200; LUT-Size: 4 & 56,738 & 184 & 4,880.07 s (81.33 min) \\ %AIG Opt. ! % 04
\bottomrule
\end{tabular}
}
\end{sc}
% \end{small}
\end{center}
% \vskip -0.1in
\end{table*}




% -------------------------------------------------------
\begin{table*}[ht]
\caption{Results of \textbf{LogicNet} as intermediate step with the logic being quantized to \textbf{32 total bits and 16 fractional bits}. The column-wise ``winner" is marked in bold.}
\label{lgn_thirtytwototal_results}
\vskip 0.15in
\begin{center}
\begin{sc}
\scalebox{0.8}{
\begin{tabular}{ccccccc}
\toprule
Depth & Width & LUT-Size & AIG Nodes & AIG Levels & Logic Accuracy (\%) \\
\midrule
2 & 50 & 4 & \textbf{207,153} & \textbf{422} & 54.17 \\
2 & 100 & 4 & 208,996 & 431 & 54.17 \\
2 & 200 & 4 & 858,284 & 493 & 56.33 \\
2 & 50 & 6 & 1,519,223 & 511 & 47.33 \\
2 & 100 & 6 & 1,437,803 & 497 & 54.50 \\
2 & 200 & 6 & 756,667 & 453 & 54.17 \\
2 & 50 & 8 & 984,625 & 454 & 51.50 \\ 
2 & 100 & 8 & 948,956 & 454 & 51.17 \\ 
2 & 200 & 8 & 1,031,077 & 450 & 53.67 \\ 
% \midrule
3 & 50 & 4 & 1,744,909 & 515 & 46.83 \\ 
3 & 100 & 4 & 1,590,823 & 514 & 54.17 \\ 
3 & 200 & 4 & 716,599 & 453 & 53.50 \\ 
3 & 50 & 6 & 238,3425 & 512 & 53.00 \\ 
3 & 100 & 6 & 2,385,562 & 517 & 53.50 \\ 
3 & 200 & 6 & 1,338,098 & 464 & 55.33 \\
3 & 50 & 8 & 1,333,842 & 462 & 46.00 \\
3 & 100 & 8 & 1,339,410 & 463 & 53.17 \\
3 & 200 & 8 & 1,345,170 & 465 & 54.33 \\
% \midrule
4 & 50 & 4 & 1,286,186 & 454 & \textbf{64.33} \\ 
4 & 100 & 4 & 1,288,754 & 461 & 56.67 \\ 
4 & 200 & 4 & 1,288,886 & 458 & 40.83 \\ 
4 & 50 & 6 & 1,343,026 & 466 & 47.50 \\ 
4 & 100 & 6 & 1,353,394 & 466 & 52.83 \\
4 & 200 & 6 & 1,360,466 & 467 & 53.50 \\
4 & 50 & 8 & 1,341,298 & 463 & 56.67 \\ 
4 & 100 & 8 & 1,349,522 & 470 & 51.33 \\ 
4 & 200 & 8 & 1,361,810 & 465 & 60.83 \\
\bottomrule
\end{tabular}
}
\end{sc}
\end{center}
\end{table*}

% -------------------------------------------------------
\begin{table*}[ht]
\caption{Results of \textbf{random forest} as intermediate step with the logic being quantized to \textbf{8 total bits and 6 fractional bits}. The column-wise ``winner" for a setting with and without AIG optimization is marked in bold.}
\label{rf_thirtytwototal_results}
\vskip 0.15in
\begin{center}
\begin{sc}
\scalebox{0.8}{
\begin{tabular}{cccccc}
\toprule
Estimators & Max. Depth & AIG Nodes & AIG Levels & Logic Accuracy (\%) \\
% \midrule
2 & 5 & \textbf{1,660,911} & \textbf{506} & 54.67 \\
2 & 10 & 2,688,533 & 530 & 52.50 \\
2 & 15 & 2,389,484 & 541 & 51.67 \\
% \midrule
3 & 5 & 1,865,767 & 519 & \textbf{55.67} \\
3 & 10 & 4,164,037 & 592 & 48.50 \\
3 & 15 & 2,934,422 & 553 & 51.67 \\
% \midrule
4 & 5 & 3,153,180 & 600 & 53.33 \\
4 & 10 & 3,458,848 & 565 & 50.00 \\
4 & 15 & 3,469,420 & 564 & 52.67 \\
\bottomrule
\end{tabular}
}
\end{sc}
\end{center}
\end{table*}
